# Supplementary material for: TRIGO: Benchmarking Formal Mathematical Proof Reduction for Generative Language Models
Source: arXiv:2310.10180 source file (2023-10-24)
Supplement: Supplementary file 1 [file program_appendix.tex]

\begin{table*}[!htb]
\centering
\scalebox{1.0}{
\begin{tabular}{l} 
\hline
\textbf{Algorithm 1} Theorem Generator \\
\hline 
1: function GENERATE\_THEOREM(len of step $\mathcal{L}$, rule list $\mathcal{R}$) \\
2: \quad Randomly select a rule from $\mathcal{R}$:$r_0 \sim Uniform(\mathcal{R})$. \\
3: \quad Initialize the parameters $X$, $Y$, $K$ in ${r_0}$ and get its initialization state in lean and expression: $P_{state}, eq_0 \sim Initialize({r_0})$. \\
4: \quad for $t \leftarrow 1$ to $200$ do \\
5: \quad \quad \quad Randomly select a rule from $\mathcal{R}$:$R_t \sim Uniform(\mathcal{R})$. \\
6: \quad \quad \quad Match the formula $R_l$ on the left side of the ${R_t}$ equation with the formulas $e_l$ and $e_r$ on the left and right sides of $eq_{t-1}$,\\ 
\quad \quad \quad \quad  and return the matching parameters. Since there are multiple matches, a matching result can be randomly selected:\\ 
\quad \quad \quad \quad $Para_l \leftarrow Rule\_Matching(R_l, e_l)$. \\ 
\quad \quad \quad \quad $Para_r \leftarrow Rule\_Matching(R_l, e_r)$.\\
7: \quad \quad \quad If $Para_l$ or $Para_r$ is not empty, substitute the parameters into $R_t$:\\
\quad \quad \quad \quad $R_p \leftarrow Parameter\_Replacement(R_l, Para_l)$, if $Para_l$ is not NULL.  \\
\quad \quad \quad \quad $R_p \leftarrow Parameter\_Replacement(R_l, Para_r)$, elif $Para_r$ is not NULL. \\

8: \quad \quad \quad Perform the equation replacement operation:\\
   \quad \quad \quad \quad $eq_t \leftarrow Equation\_Replacement(eq_{t-1}, R_p, R_r)$.\\
9: \quad \quad \quad Get the tactics corresponding to the rule: \\
   \quad \quad \quad \quad $tactics_{R_t} \leftarrow R_t.Get\_Tactics(eq_{t-1}, R_p, R_r)$.\\ %axiom.get_tactics(substitution_dict, substitution_dict["left"], substitution_dict["right"])
10: \quad \quad \quad Obtain the tactic of adjusting the cross terms in $eq_{t-1}$: \\
\quad \quad \quad \quad $tactics_{term} \leftarrow Get\_Cross\_Term(e_l, R_p)$, if $Para_l$ is not NULL.  \\
\quad \quad \quad \quad $tactics_{term} \leftarrow Get\_Cross\_Term(e_r, R_p)$, elif $Para_r$ is not NULL.\\
11:\quad \quad \quad Apply $tactics_{R_t}$ and $tactics_{terms}$ to lean-gym to obtain the GOAL$_{lean}$ in lean: \\
\quad \quad \quad \quad GOAL$_{lean}$ $\leftarrow Apply\_Tactics(tactics_{term}, tactics_{R_t})$. \\
12: \quad \quad \quad \quad end for \\
8: \quad end for \\
9: return $C_L, P$ \\
10: end function\\
\hline
\end{tabular}
}  \vspace{-4mm}
    \caption{The rules used and their corresponding formulas. Notations (2/3)}
    \label{tab:program}
    \vspace{-4mm}
\end{table*}
